# Supplementary material for: A Faster Parameterized Algorithm for Treedepth
Source: arXiv:1401.7540 source file (2014-08-20)
Supplement: Supplementary file 1 [file appendix.tex]

In this appendix, we define some of the problems that we mention 
in this paper.  

\begin{defproblem}{Treewidth}
	Input:   & A graph $G$ and a positive integer $\ell$.  \\
	Problem: & Is the treewidth of~$G$ at most $\ell$? 
\end{defproblem}

\begin{defproblem}{Pathwidth}
	Input:   & A graph $G$ and a positive integer $\ell$.  \\
	Problem: & Is the pathwidth of~$G$ at most $\ell$? 
\end{defproblem}
